# Supplementary material for: Learning Efficient Surrogate Dynamic Models with Graph Spline Networks
Source: arXiv:2310.16397 source file (2023-10-25)
Supplement: Supplementary file 1 [file Z_supplemental_experiment.tex]

\section{Supplemental Experiment}

\subsection{Ocean weather dataset}
\label{subsec:supplemental-experiment-dataset}

\subsection{Experiment setup}
\label{subsec:supplemental-experiment-setup}

\subsection{Result and discussion}
\label{subsec:supplemental-experiment-result}
\begin{table}[ht!]
    \centering
    \caption{Mean square error (MSE) propagation at different time stamps in seconds. Runtimes consider model inference for the full rollouts. Smaller is better ($\downarrow$). Best in \textbf{bold}; second \underline{underlined}.}
    \vspace{4mm}
    \resizebox{\textwidth}{!}{
    \begin{tabular}{llrccccccc}
    \toprule
    
    % Header rows
    % \multicolumn{1}{c}{Method}
    Dataset & Metric & & \multicolumn{4}{c}{Baselines} & \multicolumn{3}{c}{\ourmodel{}}
    \\
    \cmidrule(lr){4-7} \cmidrule(lr){8-10}
    & & & GCN & GNC+MLP & GEN & \baseline{} & \baseline{+OSC(Post)} & \baseline{+OSC} & \baseline{+OSC+Adaptive}  
    \\
    \midrule
    
    % Heat Equation
    \multirow{7}{*}{Ocean} & \multirow{5}{*}{MSE {\footnotesize ($\times10^{-1}$})}  
      & 1(s) & $2.23\pm0.14$ & $2.02\pm0.16$ & $\underline{1.33}\pm0.05$ & $1.45\pm0.08$ & $1.56\pm0.09$ & $1.48\pm0.07$ & $\mathbf{1.31}\pm0.10$ \\
    & & 2(s) & $2.98\pm0.21$ & $2.57\pm0.20$ & $\underline{1.65}\pm0.11$ & $2.04\pm0.12$ & $1.98\pm0.13$ & $1.87\pm0.11$ & $\mathbf{1.52}\pm0.13$ \\
    & & 3(s) & $3.55\pm0.40$ & $2.91\pm0.43$ & $2.47\pm0.21$ & $2.67\pm0.27$ & $2.55\pm0.25$ & $\underline{2.37}\pm0.20$ & $\mathbf{2.03}\pm0.28$ \\
    & & 4(s) & $4.67\pm0.97$ & $3.89\pm0.70$ & $3.37\pm0.33$ & $3.41\pm0.39$ & $3.02\pm0.37$ & $\underline{2.88}\pm0.31$ & $\mathbf{2.57}\pm0.42$ \\
    & & 5(s) & $6.02\pm1.12$ & $5.23\pm0.98$ & $4.55\pm0.52$ & $4.75\pm0.61$ & $3.82\pm0.49$ & $\underline{3.61}\pm0.38$ & $\mathbf{3.34}\pm0.44$ \\ 
    \cmidrule[0.1pt]{2-10}
    & Rollout steps \# & & 50 & 50 & 50 & 50 & 12 & 12 & 12 
    \\
    & Runtime [s] & & $3.56\pm0.15$ & $3.38\pm0.13$ & $7.11\pm0.31$ & $7.15\pm0.25$ & $1.61\pm0.12$ & $\mathbf{1.44}\pm0.09$ & $\underline{1.57}\pm0.11$ 
    \\ 
    \bottomrule
    \end{tabular}}
    \label{tab:ocean-result}
\end{table}
